# Supplementary material for: Electrolytes structure near electrodes with molecular size roughness
Source: arXiv:2102.10190 source file (2021-05-19)
Supplement: Supplementary file 1 [file appendix_capacitance.tex]

\section{Calculation of the capacitance properties}
\subsection{flat electrode}
To define the parameters $\gamma_i=v_i \rho^0$ we consider 1050 cations and 1050 anions inside the volume $11^2\times \SI{24 }{nm^3}$, similarly with work \cite{fedorov2008ionic}. Therefore the parameters $\gamma_1=0.4$ and $\gamma_2=0.05$ described the MD simulations shown in Fig.~2 correspond to $d_1=$
\subsection{rough electrode}
\begin{figure*}[b]
    \centering
    \includegraphics[width=0.45 \textwidth]{figures/charge_rough.png}
    \includegraphics[width=0.45 \textwidth]{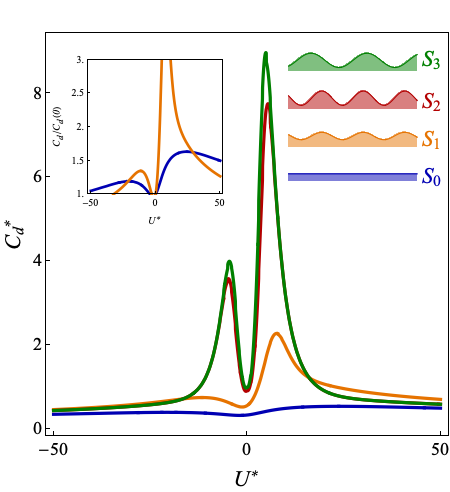}
    \caption{
    (a) The half pore charge of ions mixture with $d_1=4/3 d_2$ accounting for the various surface geometer. Inset shows the size-relations of the considered surfaces. 
    (b) The differential capacitance of binary mixture with $d_1=4/3 d_2$ accounting for the various surface geometer. Inset shows the larger scale of DC flat and insignificantly rough surfaces.
    }
    \label{fig:charge_rough}
\end{figure*}
